# Supplementary material for: Block-diagonal Hessian-free Optimization for Training Neural Networks
Source: arXiv:1712.07296 source file (2017-12-20)
Supplement: Supplementary file 1 [file supplemental.tex]

% \noindent {\Large \textbf{Supplementary Material}}
% \section{Conjugate Gradient Algorithm}
% \begin{algorithm}[th]
% \caption{Conjugate Gradient Algorithm}\label{alg:CG}

% \textbf{Input}: $\bb, \bA$, a starting value $\bx$, a maximum number of iterations ITER\_MAX; \\
% Note: Here for Hessian free method, $\bb = - \nabla_w$ is the minus gradient, which can be obtained from ``loss.backward()''. $\bA$ is the Hessian w.r.t the parameter of the network. Starting value $\bx$ can be initialized as $\bzero$.

% \textbf{Initialization}: 
% \begin{flalign}
% &i\gets 0\\
% &\br \gets \bb - \bA \bx\\
% &\bd \gets \br\\
% &\delta_{new} \gets \br^T\br\\
% &\epsilon = 0.001, \quad \delta_0 =\delta_{new}
% \end{flalign}
%  \textbf{Loop}:  While $i< \text{ITER\_MAX}$ and $\delta_{new} > \epsilon\cdot \delta_0$:
%  \begin{flalign}
%  &\bq \gets \bA\bd\\
%  &\alpha \gets \frac{\delta_{new}}{\bd^T\bq}\\
%  & \bx \gets \bx + \alpha \bd\\
%  & \br \gets \br - \alpha \bq\\
%  & \delta_{old} \gets \delta_{new}\\
%  & \delta_{new} \gets \br^T\br \\
%  & \bd \gets \br + \frac{\delta_{new}}{\delta_{old}} \cdot \bd \\
%  & i \gets i + 1
%  \end{flalign} 
%  \textbf{Output}: $\bx$.
% \end{algorithm}
% In the conjugate gradient procedure, $\bb=- \nabla_w()$ and $\bA$ is the Hessian or Gauss-Newton matrix.
% The main computation comes from the matrix vector product. Next we briefly discuss the implementation the Hessian vector product or Gauss-Newton vector product by using the $\cR\{\cdot\}$ operator.


% \section{The $\cR\{\cdot\}$ Operator}
% There is a way exactly computes $\bH\bv$, rather than approximating it. The $\bH\bv$ is defined as a directional derivative, 
% \begin{flalign}
% \bH\bv = \lim_{\alpha \to 0} \frac{\nabla_{\bw} (\bw + \alpha \bv) - \nabla_{\bw} (\bw)}{\alpha}
% = \frac{\partial}{\partial \alpha}\nabla_{\bw} (\bw + \alpha \bv)\big|_{\alpha = 0}
% \end{flalign}
% Next, we define the operator
% \begin{flalign}
% \cR_{\bv} \{f(\bw)\} := \frac{\partial}{\partial \alpha} f(\bw + \alpha \bv)\big|_{\alpha = 0}
% \end{flalign}
% Thus $\bH \bv = \cR_{\bv} \{\nabla_{\bw}(\bw)\} $. (Without ambiguity, we write $\cR \{\cdot\}$ instead of $\cR_{\bv} \{\cdot\}$.) Because $\cR \{\cdot\}$ is a differential operator, it obeys the usual rules for differential operators, such as:
% \begin{flalign}
% \cR \{cf(\bw)\}  &= c\cR \{f(\bw)\} \\
% \cR \{f(\bw) + g(\bw)\}  &= \cR \{f(\bw)\} + \cR \{g(\bw)\} \\
% \cR \{f(\bw) g(\bw)\}  &= \cR \{f(\bw)\}g(\bw) + f(\bw)\cR \{g(\bw)\} \\
% \cR \{f(g(\bw))\}  &= f'(g(\bw))\cR \{g(\bw)\}
% \end{flalign}
% Also note that
% \begin{flalign}
% \cR\{\bw\} = \bv
% \end{flalign}
% In order to compute the Hessian/Gauss-Newton vector product for the feedforward neural network, please refer to \citep{martens2012training}. Next we provide an example of computing the Gauss-Newton vector product for the LSTM network.
% % For the feedforward neural network, we define 
% % \begin{flalign*}
% % &\bs_i \gets \bW \ba_{i-1} +\bb \\
% % &\ba_i \gets \phi(\bs_i)	\\
% % & i =1, \ldots, l 	\\
% % &\ba_0 \gets \text{input} 
% % \end{flalign*}

% % \begin{algorithm}[th]
% % \caption{Compute $\bH \bv$}\label{alg:Hv}

% % \textbf{Input}:    $(\cR\bW_1, \ldots, \cR\bW_l, \cR\bb_1, \ldots, \cR\bb_l) \gets \bv$,\\
% % $\cR\ba_0 \gets \bzero$
% % \vspace{6mm}

% % \# {Forward pass}

% % \hspace{1.5cm}
% %  \textbf{for all $i$ from $1$ to $l$ do}:  
% %  \begin{flalign*}
% %  &\cR \bs_i \gets \cR \bW_i \ba_{i-1} + \bW_i \cR\ba_{i-1} +\cR\bb_i\\
% %  &\cR \ba_i \gets \cR \bs_i \phi'_i(\bs_i)
% %  \end{flalign*}
% % \hspace{1.5cm} \textbf{end}
% %  \vspace{6mm}
 
% % \# {Apply Hessian of the loss w.r.t the top layer}
% %  \begin{flalign*}
% %  \cR \cD\ba_l \gets \cR\left( \frac{\partial L(y,\bz}{\partial \bz}\Big|_{\bz=\ba_l}\right) = \frac{\partial^2 L(y, \bz)}{\partial \bz^2} \Big|_{\bz= \ba_l} \cdot \cR{\ba_l}
% %  \end{flalign*}
% %  \vspace{6mm}
 
% %  \# {Backward pass}
 
% %  \hspace{1.5cm}\textbf{for all $i$ from $l$ to $1$ do}:  
% %  \begin{flalign*}
% %  &\cR \cD\bs_i \gets \cR \cD \ba_i \odot \phi'_i (\bs_i) + \cD \ba_i \odot \cR(\phi'_i(\bs_i)) \\
% %  &\cR\cD\bW_i \gets \cR\cD\bs_i\ba_{i-1}^T + \cD\bs_i \cR\ba_{i-1}^T \\
% % &\cR\cD\bb_i \gets \cR\cD\bs_i\\
% % & \cR\cD\ba_{i-1} \gets \cR \bW_i^T\cD\bs_i + \bW_i^T\cR\cD\bs_i 
% %  \end{flalign*}
% %  \hspace{1.5cm}\textbf{end}
% % \vspace{6mm}

% %  \textbf{Output}: $\bH\bv \gets (\cR\cD\bW_1, \ldots, \cR\cD\bW_l, \cR\cD\bb_1, \ldots, \cR\cD\bb_l)$.
% % \end{algorithm}

% % Generalize the R operator to Gauss-Newton Matrix

% % \begin{algorithm}[th]
% % \caption{Compute $\bG \bv$}\label{alg:Gv}

% % \textbf{Input}:    $(\cR\bW_1, \ldots, \cR\bW_l, \cR\bb_1, \ldots, \cR\bb_l) \gets \bv$,\\
% % $\cR\ba_0 \gets \bzero$
% % \vspace{6mm}

% % \# {Forward pass}

% % \hspace{1.5cm}
% %  \textbf{for all $i$ from $1$ to $l$ do}:  
% %  \begin{flalign*}
% %  &\cR \bs_i \gets \cR \bW_i \ba_{i-1} + \bW_i \cR\ba_{i-1} +\cR\bb_i\\
% %  &\cR \ba_i \gets \cR \bs_i \phi'_i(\bs_i)
% %  \end{flalign*}
% % \hspace{1.5cm} \textbf{end}
% %  \vspace{6mm}
 
% % \# {Apply Hessian of the loss w.r.t the top layer}
% %  \begin{flalign*}
% %  \cR \cD\ba_l \gets \cR\left( \frac{\partial L(y,\bz}{\partial \bz}\Big|_{\bz=\ba_l}\right) = \frac{\partial^2 L(y, \bz)}{\partial \bz^2} \Big|_{\bz= \ba_l} \cdot \cR{\ba_l}
% %  \end{flalign*}
% %  \vspace{6mm}
 
% %  \# {Backward pass}
 
% %  \hspace{1.5cm}\textbf{for all $i$ from $l$ to $1$ do}:  
% %  \begin{flalign*}
% %  &\cR \cD\bs_i \gets \cR \cD \ba_i \odot \phi'_i (\bs_i)  \\
% %  &\cR\cD\bW_i \gets \cR\cD\bs_i\ba_{i-1}^T  \\
% % &\cR\cD\bb_i \gets \cR\cD\bs_i\\
% % & \cR\cD\ba_{i-1} \gets  \bW_i^T\cR\cD\bs_i 
% %  \end{flalign*}
% %  \hspace{1.5cm}\textbf{end}
% % \vspace{6mm}

% %  \textbf{Output}: $\bG\bv \gets (\cR\cD\bW_1, \ldots, \cR\cD\bW_l, \cR\cD\bb_1, \ldots, \cR\cD\bb_l)$.
% % \end{algorithm}

% % \newpage

% For LSTM network, 
% \begin{flalign*}
% &\bi_t = \sgm(\bW_{ii} \bx_t + \bb_{ii} + \bW_{hi} \bh_{t-1} + \bb_{hi})\\
% &\bff_t = \sgm(\bW_{if} \bx_t + \bb_{if} + \bW_{hf} \bh_{t-1} + \bb_{hf})\\
% &\bg_t = \sgm(\bW_{ig} \bx_t + \bb_{ig} + \bW_{hg} \bh_{t-1} + \bb_{hg})\\
% &\bo_t = \sgm(\bW_{io} \bx_t + \bb_{io} + \bW_{ho} \bh_{t-1} + \bb_{ho})\\
% &\bc_t = \bff_t \odot \bc_{t-1} + \bi_t \odot \bg_t\\
% & \bh_t = \bo_t \odot \tanh(\bc_t)
% \end{flalign*}
% Next, we design the algorithm to compute $\bG\bv$ for LSTM

% \begin{algorithm}[th]
% \caption{Compute $\bG \bv$ for LSTM}\label{alg:Gvlstm}

% \textbf{Input}:    %$(\cR\bW_{ii}, \cR\bW_{io}, \cR\bW_{ig} \cR\bW_{if} , \cR\bW_{hi}, \cR\bW_{ho}, \cR\bW_{hg} \cR\bW_{hf} , \cR\bb_i, \cR\bb_o, \cR\bb_g, \cR\bb_f) \gets \bv$,\\
% $(\cR\bW_{i}, \cR\bW_{o}, \cR\bW_{g} ,\cR\bW_{f} ,  \cR\bb_i, \cR\bb_o, \cR\bb_g, \cR\bb_f) \gets \bv$,\\
%  $\bx[1:t], \quad \cR\bh_0 \gets \bzero, \quad \cR\bc_0 \gets \bzero,\quad $
 
%  Denote the outputs  before activation as $\bff^s_j, \bi^s_j, \bg^s_j, \bo^s_j$, respectively.

% \vspace{2mm}

% \# {Forward pass}

% \hspace{3mm}
%  \textbf{for all $j$ from $1$ to $t$ do}:  
%  \begin{flalign*}
%  &\cR\bff_j \gets \sgm'(\bff^s_j) \odot \left(\cR\bW_{if} \bx_j + \cR\bb_{if} + \cR\bW_{hf} \bh_{j-1} + \cR\bb_{hf} + \bW_{hf}\cR\bh_{j-1}\right)\\
%  &\cR\bi_j \gets \sgm'(\bi^s_j) \odot \left(\cR\bW_{ii} \bx_j + \cR\bb_{ii} + \cR\bW_{hi} \bh_{j-1} + \cR\bb_{hi} + \bW_{hi}\cR\bh_{j-1}\right)\\
% &\cR\bg_j \gets \tanh'(\bg^s_j) \odot \left(\cR\bW_{ig} \bx_j + \cR\bb_{ig} + \cR\bW_{hg} \bh_{j-1} + \cR\bb_{hg} + \bW_{hg}\cR\bh_{j-1}\right)\\
% &\cR\bo_j \gets \sgm'(\bo^s_j) \odot \left(\cR\bW_{io} \bx_j + \cR\bb_{io} + \cR\bW_{ho} \bh_{j-1} + \cR\bb_{ho} + \bW_{ho}\cR\bh_{j-1}\right)\\
%  &\cR \bc_j \gets \cR\bff_j \odot \bc_{j-1} + \bff_j \odot \cR\bc_{j-1} + \cR\bi_j \odot \bg_{j} + \bi_j \odot \cR\bg_{j}\\
%  &\cR \bh_j \gets \cR \bo_j \odot \tanh(\bc_{j}) + \bo_j \odot \tanh'(\bc_{j})\odot \cR\bc_j 
%   \end{flalign*}
% \hspace{3mm} \textbf{end}
%  \vspace{2mm}
 
%  \# {Linear layer before softmax}
%  \begin{flalign*}
%  \cR\bz \gets \cR\bW_{fc} \bh_t + \cR\bb_{fc} + \bW_{fc} \cR\bh_t\\
%  \end{flalign*}
% \# {Apply Hessian of the loss w.r.t the top layer}
%  \begin{flalign*}
%  &\cR \cD\bz \gets \cR\left( \frac{\partial L(y,\bz)}{\partial \bz}\right) = \frac{\partial^2 L(y, \bz)}{\partial \bz^2} \cdot \cR{\bz}
%  \end{flalign*}
%  \# {Backward pass}
%  \begin{flalign*}
%  &\cR\cD\bW_{fc} \gets \cR\cD\bz \bh_t^T\\
%  &\cR\cD\bb_{fc} \gets \cR\cD\bz\\
%  &\cR\cD\bh_t \gets \bW_{fc}^T\cR\cD\bz \\
%    &\cR \cD\bc_t \gets \bzero
%  \end{flalign*}

%  \hspace{3mm}\textbf{for all $j$ from $t$ to $1$ do}:  
%  \begin{flalign*}
%  &\cR\cD \bc_{j} \gets \cR\cD \bc_{j} +  \cR\cD\bh_j \odot\bo_j \odot \tanh'(\bc_j)\\
%  &\cR\cD\bo_j \gets \cR \cD\bh_j \odot\tanh(\bc_j) \\
% &\cR\cD \bo^s_j \gets \cR\cD\bo_j \odot \sgm'(\bo^s_j) 	\quad\quad \# \; \bo_j = \sgm (\bo^s_j)\\
% & \cR\cD\bff_j \gets  \cR\cD\bc_{j}\odot\bc_{j-1} \\
% &\cR\cD\bff^s_j \gets \cR\cD\bff_j \odot \sgm'(\bff^s_j) \\
% & \cR\cD\bi_j \gets  \cR\cD\bc_{j}\odot\bg_{j} \\
% &\cR\cD\bi^s_j \gets \cR\cD\bi_j \odot \sgm'(\bi^s_j) \\
% & \cR\cD\bg_j \gets  \cR\cD\bc_{j}\odot\bi_{j} \\
% &\cR\cD\bg^s_j \gets \cR\cD\bg_j \odot \tanh'(\bg^s_j) \\
% &\cR\cD \bW_{if} \gets \cR\cD \bW_{if}  + \cR\cD\bff^s_j \bx_j^T \\
% &\cR\cD \bb_{if} \gets \cR\cD \bb_{if} + \cR\cD\bff^s_j\\
% &\cR\cD \bW_{hf} \gets \cR\cD \bW_{hf}  + \cR\cD\bff^s_j \bh_j^T  \\
% &\cR\cD \bb_{hf} \gets \cR\cD \bb_{hf} + \cR\cD\bff^s_j\\
% & \cR\cD \bW_{o} ,  \cR\cD \bb_{o} ,  \cR\cD \bW_{g} , \cR\cD \bb_{g} , \cR\cD \bW_{i} , \cR\cD \bb_{i} \\
% &\cR\cD\bh_{j-1} \gets \bW_{hi} ^T{\cR\cD\bff^s_j}   +  \bW_{hi} ^T\cR\cD{\bi^s_j}  + \bW_{ho} ^T\cR\cD{\bo^s_j}  +  \bW_{hg} ^T\cR\cD{\bg^s_j} \\
% &\cR\cD \bc_{j-1} \gets \cR\cD \bc_j \odot \bff_j
%  \end{flalign*}
%  \hspace{1cm}\textbf{end}
% \vspace{2mm}

%  \textbf{Output}: $\bG\bv \gets (\cR\cD\bW_{i}, \cR\cD\bW_{o}, \cR\cD\bW_{g}, \cR\cD\bW_{f} ,  \cR\cD\bb_i, \cR\cD\bb_o, \cR\cD\bb_g, \cR\cD\bb_f)$.
% \end{algorithm}
